# Supplementary material for: In- and Out-of-Distribution Generalization of Reasoning in Multimodal LLMs for Simple Visual Planning Tasks
Source: arXiv:2602.15460 source file (2026-11-25)
Supplement: Supplementary file 1 [file A_appendix_overview.tex]

\clearpage
\setcounter{page}{1}
\maketitlesupplementary

We give an overview over the contents of the Appendix.

\begin{itemize}
    \item 
\end{itemize}
